# Supplementary material for: Between Randomness and Arbitrariness: Some Lessons for Reliable Machine Learning at Scale
Source: arXiv:2406.09548 source file (2024-08-12)
Supplement: Supplementary file 2 [file 10-app-emergent-intro.tex]

Optimization is a problem formulation technique that lies at the core of multiple engineering domains.
Given some fixed or limited resource, we can model its usage to effectively solve a problem. The optimal solution is the one that either minimizes some cost function or maximizes some utility function --- functions that measure how well the model performs on a particular objective. Often there is more than one objective to satisfy simultaneously, and those objectives can be in tension with one another. In this case, it is possible to pose this problem as optimizing a trade-off \cite{yang2010optimization}.

For an intuitive example, consider a company that has a fixed amount of steel; the company uses the steel to build cars and planes, which it then sells to earn a profit. The company has to decide how to allocate the steel to maximize that profit and can formulate the decision as an optimization problem. The blue curve in Figure \ref{fig:optimization} models possible ways to do this optimally; picking a specific point on the curve corresponds to the company's choice for how to balance the trade-off between how many cars and how many planes to produce.

\begin{figure}[ht]
    \centering
    \includegraphics[width=0.5\linewidth]{figure/91-emergent/optimization.pdf}
    \caption{Illustrating a trade-off. Given a fixed amount of steel, a company can build a combination of cars and planes. To optimally utilize the steel for maximizing profit, it can manufacture any point on the blue curve. Any combination above the curve is not possible because there is insufficient steel; any below is suboptimal because the same amount of steel could either produce more cars or more planes.}
    \label{fig:optimization}
\end{figure}

Optimization science has informed much of the last decade's spectacular spate of statistical machine learning (ML) publications. It is at the core of how many ML algorithms learn. For example, learned classifiers use training data examples to fit a curve that optimizes for both classifying those examples correctly and generalizing to new, unclassified examples~\cite{bishop1995mlbook, hastie2009statistical}. This process of automating classification decisions has in the past been framed as optimal in another sense; automation brought with it the hope of rooting out the human (suboptimal) whims of decisionmaking---of eliminating the ugliest human biases, such as sexism and racism, that afflict high-impact decision processes. Yet, as has been well-documented, this hope cannot be passively realized merely by substituting humans with automated decision agents. Issues with biased data and biased model selection processes can in the worst case magnify, rather than replace, human biases~\cite{abebe2020social, forde2021model, selbst2019abstraction}.

In response, there has been a widespread push to actively engineer \emph{algorithmic fairness}. This has become remarkably urgent as automated decision systems are being deployed in domains that have a significant impact on the quality of human life---in deciding judicial bail conditions, loan allocation, college admissions, hiring outcomes, COVID vaccine distribution, etc.,~\cite{monahan2016risk, barocas2016data, ajunwa2020hiring, angwin2016machine}. Models no longer just need to be correct; they also need to be fair.

It has become common to position accuracy in opposition to fairness and to formalize a mathematical trade-off between the two. For example, in the context of criminal justice and bail decisions, the accuracy of decisions has been framed as how to best ``maximize public safety," in contrast to satisfying ``formal fairness constraints" that aim to reduce racial disparities in decision outcomes \cite{corbettdavies2017cost}. This kind of problem formulation is the norm in a growing area of research, in which the trade-off between fairness and accuracy in ML is considered ``inherent" or ``unavoidable." Prior work suggests various ways of implementing the trade-off: At best, under particular conditions, the tension between the two can be dissolved to achieve both; at worst, fairness is sacrificed in favor of accuracy, while the remaining cases fall somewhere in the middle~\cite{dutta2020tradeoff, chen2018tradeoff, bakker2019active, menon2018cost, noriegacampero2019active}.

\subsection*{Our Contribution}
Our work looks both at and beyond the fairness-accuracy trade-off, drawing from prior critiques of algorithmic fairness and studies of sociotechnical systems. We examine the \emph{choice}---and our work here will show that it is a choice, not a requirement---to model assumptions that cast fairness in direct opposition to accuracy. Regardless of the particulars of specific implementations, this framing does not just involve math, but also implicates normative concerns regarding how to value fairness and accuracy both independently and in relation to each other~\cite{flanagan2014values, friedman2019values}. 

Our contribution is to extract and explore patterns of these concerns across trade-off scholarship that arise at three different stages: the initial modeling assumption to treat accuracy and fairness together in an optimization problem, the move from abstract framing to concrete problem formulation, and the ``optimal solutions" that result from those formulations. More specifically, we examine how the choice to operationalize the relationship between fairness and accuracy using the language of optimization inherently puts the two in conflict, rather than leaving open the legitimate possibility for them to actually be in accord. We discuss how this choice fails to take full account of social criteria when drawing the boundaries of a problem~\cite{selbst2019abstraction}, and relates to broader trends of techno-``solutionism,'' in which math is (mistakenly) bestowed special authority to ``solve'' social problems~\cite{abebe2020social}.

Beyond  these overarching framing assumptions, there are other underlying, unexamined normative assumptions (not just explicit mathematical ones) that take root in how the trade-off is formalized: That strict notions of mathematical equality can model fairness, that it is possible to measure the accuracy and fairness of decisions independent from historical context, and that collecting more data on marginalized individuals --- a practice called \emph{active fairness} --- is a reasonable solution to mitigate the effects of the trade-off.

If we take the time to clarify these implicit assumptions, we note that the conclusions that follow can actually perpetuate unfairness: The mathematical proofs may be sound --- a particular choice of fairness metric may even be optimized --- but the implicit normative assumptions and accompanying broader normative results suggest that these methods will not ensure fairer outcomes in practical applications. In summary, we argue that
\begin{itemize}
    \item Using the language of optimization situates fairness and accuracy in intrinsic opposition, generally privileging the latter over the former and necessarily foreclosing the possibility of examining the ways they can instead reinforce each other (Section \ref{app:sec:emergent:sociotechnical}).
    \item Underlying mathematical assumptions bring unexamined normative dimensions, which can actually result in emergent unfairness (Section \ref{app:sec:emergent:assumptions}).
    \item In light of these observations, algorithmic fairness researchers will conduct more robust research if they first clarify their normative assumptions (Section \ref{app:sec:emergent:resolution}).
    \item Due to the extent of emergent unfairness from conceiving of fairness and accuracy in trade-off, it is worth revisiting this formulation altogether (Section \ref{app:sec:emergent:conclusion}).
\end{itemize}
