# Supplementary material for: Between Randomness and Arbitrariness: Some Lessons for Reliable Machine Learning at Scale
Source: arXiv:2406.09548 source file (2024-08-12)
Supplement: Supplementary file 3 [file 20-app-emergent-prelim.tex]

\section{The Fairness-Accuracy Trade-Off} \label{app:sec:emergent:preliminaries}

We begin by providing the background necessary for understanding the problem formulation of the fairness-accuracy trade-off. Before clarifying what the trade-off actually characterizes, we address each component in turn, summarizing common quantifiable metrics that ML researchers map to the values of ``accuracy'' and ``fairness.''

\subsection{Accuracy Metrics} \label{app:sec:emergent:accuracy}

In brief, \emph{accuracy} measures how often a ML model correctly predicts or infers a decision outcome after training. So, to understand accuracy, we need to understand how ML models are trained. For the classification problems that dominate much of the fairness literature, training the model usually entails fitting a curve to a set of training data points for which classification labels are already known. After training, when supplied with a previously-unseen data point, the model can infer the classification label for that data point. For example, in building a model that infers whether or not to grant an applicant a loan, the curve-fitting training process occurs with past data concerning loan-granting decisions; inference corresponds to the model receiving a new loan applicant's data and classifying whether that applicant should receive a loan or not --- a decision ultimately corresponding to whether or not the loan-granting institution believes the applicant will repay or default on the loan.

A model's accuracy tends to be measured during a validation process in between training and inference. Rather than using all labeled data for training, researchers reserve a portion to validate how well the trained model classifies unseen data points with known classification labels. In other words, accuracy is often a measure of \emph{label alignment}: It is the percentage of correctly classified validation data points, where correctness is determined by whether the model's classification decision matches the known label. There are other metrics that researchers use, such as Chernoff information \cite{dutta2020tradeoff}; however, label alignment is a popular accuracy metric, in part due to its simplicity.

This simplicity can be misleading, both in terms of what the math is actually measuring and the normative implications of that measurement. The broader algorithmic fairness community (and corresponding community of critics) has paid ample attention to this issue in relation to fairness \cite{binns2018phil, selbst2019abstraction, powles2018bias, abdurahman2019response}; however, in fairness-accuracy trade-off literature, where accuracy is also explicitly centered as a value, parallel analyses of accuracy have been relatively sparse.  We examine this in Section \ref{app:sec:emergent:assumptions}; for now, we emphasize that something as simple as a percentage metric can raise normative concerns \cite{forde2021model}.

One can see this from work in the broader ML community, in which accuracy issues often get cast as a problem of \emph{label bias}: The classification labels in the training and validation data can be incorrect, in terms of some abstract notion of ``ground truth.''\footnote{The implications of ``true'' classification, including the simplifying assumptions that inform such classification, are out of scope for our purposes. We refer the reader to the rich literatures in sociology and science \& technology studies on categorization and classification, notably Velocci~\cite{velocci2021diss} and Bowker \& Star~\cite{bowker1999sorting}.} As an innocuous example, consider a labeled image dataset of dogs and cats. The individual that labeled the dataset incorrectly (though perhaps understandably) mis-labeled Pomeranians as cats. This mis-labeling in turn leads the learned ML model to mistakenly identify Pomeranians as cats. 

The results of mis-labeling can be devastating for applications that impact human lives. Consider again an automated decision system that grants and denies loan applications. In the US, systemic racism against Black loan applicants, specifically manifested in the practice of redlining, has entailed denying loans to qualified Black applicants. These applicants, in terms of ``ground truth'' should have been granted loans, but were instead intentionally marked as likely defaulters. As with the example above, this mis-labeling would lead to inaccurate classification. The models trained on that data would mistakenly identify Black non-defaulters as defaulters --- a mis-classification that could be used to wrongfully deny a loan.\footnote{We have simplified this example, which also involves using zip code as a proxy for race, to make our point that mis-labeled data impact the accuracy of trained models.} Unlike the former example, this one involves intentional mis-labeling; however, it is worth noting that even if the mis-labeling were unintentional, it would have the same effect on classification decisions. Regardless of intention, the impact would be the same. Either way, the learned model would systematically, incorrectly classify Black individuals as defaulters.

\subsection{Fairness Metrics} \label{app:sec:emergent:fairness}

Algorithmic \emph{fairness} has dozens of mathematical definitions that can inform optimization problem formulation.\footnote{Similar to our discussion of accuracy and classification, our work will not focus on the normative limits of defining fairness mathematically, such as the challenges of formulating fairness problems that account for intersectional protected identities \cite{selbst2019abstraction, chen2018tradeoff, dwork2018decoupled, buolamwini2018gender, kroll2017aa, hoffman2019fairness} and how many fairness definitions reflect \emph{what we ought to believe} instead of (the arguably more useful, from a policy perspective) \emph{what we ought to do} \cite{hellman2019fairness}.} All definitions, regardless of the specifics, involve some treatment of \emph{protected attributes}, such as race and sex, along which decision outcomes can be evaluated for ``fair'' treatment. Broadly speaking, there are two families of fairness metrics: Those that measure individual-focused fairness and those that evaluate it in terms of groups defined by protected attributes.

Individual fairness, as the name suggests, centers analyzing automated decisions in terms of the individual \cite{dwork2012fairness, joseph2016rawls, bakker2019active}. %For example, counterfactual fairness deems a decision to be fair toward an individual if it is the same regardless of the individual's membership in a particular demographic group \cite{kusner2017counterfactual}.
In contrast, group fairness centers demographic group membership and typically aims to ensure that membership in a protected class does not correlate with decision outcomes \cite{dwork2018decoupled, chen2018tradeoff}. A particularly popular metric is Hardt et al.~\cite{hardt2016equality}'s formulation of \emph{equality of opportunity}, which in essence only requires that there is no discrimination based on demographics for those assigned the positive classification. For the example of granting loans, paying back the loan is the positive class and defaulting is the negative class. Equality of opportunity corresponds to making sure that the rate of mistakenly classifying non-defaulters as defaulters is similar across demographic groups. We discuss this further in Section \ref{app:sec:emergent:assumptions}; for now, it is important to note that \emph{this formulation is inextricably tied to accuracy}. Training a model to reduce mistaken negative classification directly depends on training data that contains negative labels. Those labels, however, may not align with what is correct in terms of ``ground truth'' --- e.g., Black individuals erroneously marked as defaulters.

Lastly, it is also worth noting that multiple different mathematical notions of fairness cannot be satisfied simultaneously. This incompatibility has been formalized as impossibility results \cite{kleinberg2017impossibility,chouldechova2017impossible} and has placed a more significant emphasis on how computer scientists choose which fairness metric to study \cite{friedler2016impossibility}. While these findings are extremely well-cited, they are not surprising when considering fairness beyond its mathematical definition as a metric. In a pluralistic world, values like fairness depend on the time and place in which they are defined; outside of math, different, incompatible definitions can hold simultaneously, depending on context~\cite{berlin2013crooked}.

\subsection{The ``Inherent'' Trade-Off} \label{app:sec:emergent:tradeoff}

Algorithmic fairness tends to pose accuracy and fairness in an ``inherent'' or ``unavoidable'' trade-off: An increase in fairness necessarily comes with a decrease in accuracy; increasing accuracy necessarily decreases fairness \cite{chen2018tradeoff, menon2018cost, bakker2019active, corbettdavies2017cost, dwork2018decoupled, sabato2020bounding, zhao2019inherent}. 

How did this trade-off problem formulation come about? Much of the literature that engages this trade-off does so empirically; that is, the authors perform or cite experiments that convey the intuition that a trade-off exists, so they decide that a mathematical trade-off is an appropriate way to model the problem. However, most do not characterize or quantify the trade-off theoretically. The work that has attempted theoretical treatment suggests that --- at least in theory --- the existence of the fairness-accuracy trade-off can be less rigidly described \cite{dutta2020tradeoff, wick2019revisited}. Nevertheless, the general practice in the field is to tacitly accept the trade-off as fact, regardless of the particular fairness and accuracy metrics under consideration.

Computer scientists further observe that the ramifications of this trade-off, particularly in high-stakes domains, can be significant. As a result, they sometimes wade into the murkiness of \emph{how} to optimize the trade-off implementation in specific ``sensitive'' applications. For example, several computer scientists have noted that in areas like healthcare, trade-off implementations should favor accuracy, as privileging fairness can have ``devastating'' consequences, such as missing cancer diagnoses at higher rates \cite{chen2018tradeoff, srivastava2019perceptions}.

Other researchers have posited \emph{why} this trade-off exists in the first place. For example, one popular explanation comes from Friedler et al.~\cite{friedler2016impossibility}. The authors of this paper reason that there is an ``abstract construct space'' that represents the features we actually want to measure but cannot observe (e.g., intelligence). Instead, we see features in the ``observed space'' of the actual world (e.g., SAT score), and there is a mapping from features in the construct space to features in the observed space (e.g., SAT score is the mapped feature in the observed space, standing in place for intelligence in the construct space). According to Friedler et al.~\cite{friedler2016impossibility}, the trade-off between classification accuracy and fairness exists in the real world due to ``noisier mappings'' for less privileged groups from the construct space to the observed space. They contend that this noise comes from historic differences, particularly in opportunity and representation, which makes positive and negative data points less distinguishable (in comparison to privileged groups) for the learned classifier. It is this decrease in separability that leads to less fair classification for less privileged groups. In the example of SATs, this means that the scores are less reliable in terms of conveying information about intelligence for underprivileged groups. While this posited explanation may seem reasonable, work that engages with it rarely (if ever) supports the explanation with data, as it is usually not the specific fairness problem under mathematical consideration~\cite{dutta2020tradeoff}.
