# Supplementary material for: Between Randomness and Arbitrariness: Some Lessons for Reliable Machine Learning at Scale
Source: arXiv:2406.09548 source file (2024-08-12)
Supplement: Supplementary file 4 [file 30-app-emergent-lens.tex]

\section{Applying a Sociotechnical Lens}\label{app:sec:emergent:sociotechnical}

In the field of Science and Technology Studies, the term ``sociotechnical'' is used to signal the impossibility of understanding the social world separately from the technological, and vice versa~\cite{bijker1987sociotechnical, hughes1993power, hecht2002nuclear, wajcman2004feminism}. This means that, among other things, technologies like algorithms are never separate from the systems, institutions, ideologies, cultures, and societies in which they are embedded. It also means that the choice to formulate algorithmic fairness as an optimization problem produces a particular kind of knowledge about fairness that cannot be detached from its broader social context.
In our critiques of emergent unfairness in Section \ref{app:sec:emergent:assumptions}, we explicitly examine the fairness-accuracy trade-off model as a sociotechnical system.

We are not the first to examine algorithmic fairness using the concept of a sociotechnical system. For example, 
Selbst et al.~\cite{selbst2019abstraction} use the concept of sociotechnical systems to draw attention to five pitfalls that imperil well-meaning data scientific approaches to fairness. 
One that they identify is called the ``Framing Trap,'' which the authors describe as the ``failure to model the entire system over which a social criterion, such as fairness, will be enforced.'' A sociotechnical lens, they argue, might suggest new ways for researchers to draw the boundaries of fairness problems to include social relations and dynamics that may have otherwise been excluded. 

Defining fairness and accuracy in trade-off both exemplifies falling into the Framing Trap and presents an additional set of nuanced consequences. For example, the language of defining trade-offs along a curve (Figure \ref{fig:optimization}) necessarily requires a give-and-take relationship between the factors under consideration, as those factors are cast in opposition to one another. In the fairness-accuracy trade-off, fairness and accuracy are framed as inherently competing goals, in which we must give up some of one in order to gain some of the other (even if ``some'' cannot be quantified definitively). Based on this framing, it is consistent that much of the literature uses language that describes the ``cost of fairness'' \cite{chen2018tradeoff, menon2018cost, corbettdavies2017cost, dutta2020tradeoff}, depending on where on the trade-off optimization curve a particular implementation lies. This cost, however, can be described as cutting both ways: It is similarly reasonable to talk about the ``cost of accuracy.'' Yet, with few exceptions \cite{corbettdavies2017cost}, the literature in this area chooses not to discuss costs in this way. This decision is perhaps due to the tendency within the field of ML more broadly to privilege accuracy during model design; nonetheless, this framing shifts the burden of defensibility to fairness, in the sense that it implies that fairness' ``costs'' require justification.

The particulars of the trade-off choice present additional complications. Beyond failing ``to model the entire system'', the fairness-accuracy trade-off formulation also forecloses the very reasonable possibility that accuracy is generally in accord with fairness (unless one specifies particular conditions for which it is possible to demonstrate that the trade-off does not exist \cite{dutta2020tradeoff, wick2019revisited}). In other words, a trade-off model conceals the idea that the accurate thing to do could be complementary with the fair thing to do. For example, as Hellman \cite{hellman2019fairness} notes, it is possible to view accuracy and fairness as complementary values, where the former reflects what one ``ought to believe'' and the latter reflects what one ``ought to do.'' In Section \ref{app:sec:emergent:assumptions}, we expand on how fairness and accuracy can be considered in accord \cite{friedman2019values, flanagan2008values}. Additionally, we suggest that the boundaries of the trade-off problem need to be redrawn to account for social and technical considerations \emph{in historical context}. A suitable frame for fairness research can neither be blind to past historical context nor ignore the future. 

Lastly, our analysis demonstrates some of the challenges of using trade-off and optimization tools in algorithmic fairness research. Borrowing tools from adjacent fields in computer science not only affects the results of fairness research, but it also helps to characterize the disciplinary status of fairness research itself. In this case, the operationalization of fairness as a mathematical problem helps situate questions of fairness within the realm of ``science,'' thus conferring a particular legitimacy that science connotes \cite{gieren1983boundary,porter1995trust}. Situating the fairness question as a scientific question and esconcing it in the language of trade-offs and optimization suggests that it is reasonable to try to solve for an ``optimal,'' best answer. Framing the problem as a trade-off problem to be ``solved'' using math falls under the highly-critiqued practice of technological ``solutionism''~\cite{selbst2019abstraction, abebe2020social} --- the notion that technology is uniquely capable of solving social problems. This tendency toward solutionism grants special legitimacy to algorithmic fairness research, legitimacy absent in other fields that have tackled but have not ``solved'' the fairness problem from a social perspective. We contend that it is unlikely that the same ideas used to solve problems of steel allocation (Figure \ref{fig:optimization}) will transfer without issue to questions of fair hiring practices. We suggest that attending to the sociotechnical context of each situation may help prevent the emergent unfairness we identify in the following sections.
