# Supplementary material for: Between Randomness and Arbitrariness: Some Lessons for Reliable Machine Learning at Scale
Source: arXiv:2406.09548 source file (2024-08-12)
Supplement: Supplementary file 5 [file 40-app-emergent-unfair.tex]

\section{Emergent Unfairness}\label{app:sec:emergent:assumptions}

Choosing to convey fairness and accuracy as a trade-off is a mathematical modeling assumption. As we discussed in Section \ref{app:sec:emergent:preliminaries}, the authors have observed a pattern in their empirical results concerning accuracy and fairness, and deem a trade-off to be a useful way to formulate the mathematical problem of characterizing the relationship between the two. As we suggest above, fairness and accuracy metrics have normative dimensions; so, too, does the modeling assumption that poses them in trade-off. 

There are also numerous, other mathematical assumptions, each which carry their own implicit normative dimensions. We observe that, based on these implicit assumptions, fairness-accuracy trade-off scholarship is plagued with gaps and oversights. These issues can lead to conclusions that \emph{actually perpetuate unfairness}. There are dozens of examples of particular assumptions specific to each paper in fairness-accuracy trade-off scholarship. It is not possible to be exhaustive regarding each mathematical assumption's corresponding normative assumptions. Instead, we isolate three patterns of implicit, unexamined assumptions in the discipline, and the emergent \emph{un}fairness that can result: Unfairness from assuming 1) strict notions of equality can substitute for fairness, 2) historical context is irrelevant when formulating the trade-off, and 3) that collecting more data on marginalized groups is a reasonable mechanism for alleviating the trade-off.

\subsection{Unfairness from Assuming Fairness = Equality}

One assumption prevalent in fairness-accuracy trade-off literature concerns how different papers choose to measure fairness. Most of the work in this subfield relies on parity-based definitions. Algorithmic fairness definitions like this effectively make the modeling assumption to represent ``fairness'' as ``equality.''\footnote{While such equality-based notions of fairness dominate the literature more generally, not just concerning the fairness-accuracy trade-off, there is a growing number of exceptions. For example, some recent work frames fairness in terms of Rawlsian social welfare~\cite{rawls1971theory,heidari2018rawls, joseph2016rawls}.} To be clear, we mean ``equality'' in the strict sense of the values of metrics being as equal as possible, by minimizing some form of measured inequality. This kind of strict equality can stand in for ``fairness'' in terms of what is actually being modeled; fairness is being framed as a problem of strict equality. This is easily discernible in the popular equality of opportunity metric (Section \ref{app:sec:emergent:preliminaries}), used in numerous trade-off papers \cite{chen2018tradeoff, dutta2020tradeoff, bakker2019active, noriegacampero2019active}, which tries to minimize discrepancies in false negative classification decisions among different demographic groups; it literally tries to make those rates as equal as possible.

However, what is fair and what is equal are not always the same thing, and framing them as equivalent can actually lead to unfair outcomes \cite{kasy2021equal}. For example, when addressing historic or systemic inequity, it can be necessary to take corrective or reparative action for some demographic groups in order to create the conditions of more-equal footing. Such actions necessarily diverge from equality in the strict mathematical sense, so strictly parity-based fairness metrics cannot capture this kind of nuance.

The ongoing debate in the United States around the fairness of affirmative action policy can help illustrate this distinction, as well as the complications that arise when defining fairness as equality. In brief, affirmative action is a social policy aimed at increasing the representation of historically marginalized groups in university student and workforce populations; it attempts to implement a fairer playing field by providing individuals from marginalized backgrounds with the chance to have the same opportunities as those from more privileged backgrounds. 

While affirmative action has existed as official policy in the US for decades \cite{kennedy1961affirmative}, it is extremely contentious.
Many Americans, who do not feel personally responsible for systemic discrimination against BIPOC\footnote{An acronym for ``Black, Indigenous, and People of Color,'' used particularly in the US and Canada.} populations, feel that affirmative action puts them at a disadvantage. They claim that the policy is unfair, and in fact is responsible for ``reverse discrimination'' \cite{budryk2020ut, newkirk2017white, pham2018harvard}. This belief comes in part from the idea that affirmative action does not lead to ``equal'' comparisons in the strictest sense --- comparing SAT scores or GPAs point for point. Instead, in the language of Friedler~\cite{friedler2016impossibility}, one could say that affirmative action attempts to repair or normalize for the ``noisy mappings'' that these scores convey for unprivileged populations in order to promote fairer outcomes.\footnote{It is also interesting to note that this controversy has found its way into the language of algorithmic fairness literature. Dwork et al. \cite{dwork2012fairness, dwork2018decoupled} use the term ``fair affirmative action'' in their work; they seem to be attempting to distinguish their notion from some imagined, alternative, unfair variant. This term is arguably redundant, since affirmative action is fundamentally about trying to promote fairer outcomes, even if that notion of fairness does not align with strict-equality-based notions in algorithmic fairness.} 

In short, the goal of affirmative action illustrates how notions of fairness and equality can diverge. The policy's existence is predicated on the notion that strictly equal treatment, without attending to past inequity, can potentially perpetuate unfairness.

\subsection{Unfairness from Assuming the Irrelevance of Context}

Fundamentally, the issue with the assumption that strict notions of equality can stand in for fairness has to do with how the assumption treats --- or rather discounts --- context. Fairness metrics like equality of opportunity are only able to evaluate the local, immediate decision under consideration. As discussed above using the example of affirmative action, this type of equality cannot accommodate reparative interventions that attempt to correct for past inequity. This similarly implicates issues with how we measure accuracy, since such metrics measure the correctness of current classification decisions in relation to past ones. We next examine this issue, as it presents fundamental contradictions in the formulation of the fairness-accuracy trade-off problem.

\subsubsection{Ignoring the Past}

As discussed in the introduction, optimization involves minimizing a loss function. In statistical terminology, minimizing the expected loss depends on the \emph{true} class labels \cite{bishop1995mlbook}. In fairness-related application domains we rarely, if ever, have access to true class labels. To return to an earlier example, Black people have systematically been denied loans in the US due to their race. In many cases, while a Black person's ``true'' label should be that they would not default on a loan, past loan-granting decisions (and therefore the corresponding data) mark them as a defaulter. This captures the problem of \emph{label bias}: Misalignment between the ``ground truth'' label and the actual, observed label in real-world data (Section \ref{app:sec:emergent:preliminaries}). In a sense, this bias is what has motivated the entire field of algorithmic fairness in the first place: Automated decision systems that do not account for systemic discrimination in training data end up magnifying that discrimination \cite{barocas2019textbook, abebe2020social}; to avoid this, such systems need to be proactive about being fair.

Label bias presents an inherent issue with how we measure accuracy: If labels are wrong, particularly for individuals in the groups for which we want to increase fairer outcomes, then there are cases where misclassification is in fact the correct thing to do. In other words, how we measure accuracy is not truly accurate.

Yet, in the fairness-accuracy trade-off literature, it is very common to assume label bias can be ignored. Much of the work in this space does not mention label bias at all, or claims that it is out of scope for the research problem under consideration \cite{chen2018tradeoff}. This presents a contradiction: Simultaneously acknowledging that labels in the observed space are noisy representations of the ground truth (i.e., there is bias in the labels), but then explicitly assuming those labels in the training data (i.e., the observed space labels) are the same as the true labels \cite{dutta2020tradeoff}.\footnote{Wick et al.~\cite{wick2019revisited} is a notable exception, acknowledging this contradiction in stark terms: ``...there is a pernicious modeling-evaluating dualism bedeviling fair machine learning in which phenomena such as label bias are appropriately acknowledged as a source of unfairness when designing fair models, only to be tacitly abandoned when evaluating them.''} In other words, because the labels are biased, the corresponding accuracy measurements that depend on them are also biased; unfairness from the past produces inaccuracy~\cite{hellman2021data}, which this work explicitly ignores in its trade-off formulation.

If accuracy measurements are conditioned on past unfairness, what is the trade-off between fairness and accuracy actually measuring? What does it mean to ``increase'' or ``decrease accuracy'' in this context? If accuracy measurements encode past unfairness for unprivileged groups, the fairness-accuracy trade-off is effectively positioning fairness in trade-off with unfairness, which is tautological. Giving validity to an accuracy metric that has a dependency on past unfairness inherently advantages privileged groups; it is aligned with maintaining the status quo, as there is no way to splice out the past unfairness on which it is conditioned. In the words of Hellman~\cite{hellman2019fairness}, this can lead to even more unfair outcomes via ``compounding injustice.'' To the best of our knowledge, no prior work has explicitly attempted to avoid this scenario --- to model and extract this past unfairness.%\footnote{No scholarship in this space, to the best of our knowledge, has attempted to put a Bayesian prior on existing unfairness. Such an approach would explicitly assume and model the existing unfairness due to a history of discrimination against certain demographics. Such modeling would not come without concern, as it would require fairness researchers to introduce a different set of mathematical modeling assumptions that carry their own normative implications.}

\subsubsection{Being Blind to the Future}

Similarly, studying specific, local classification decisions in terms of balancing fairness and accuracy does not provide insight about the more global, long-term effects that such decisions potentially have. This also presents a contradiction: Some scholarship concerning the trade-off explicitly aims to support the goals of policymakers, but policymaking by its very nature takes a long-tailed view. Current policy interventions do not just have a local impact, but rather also have desired cascading effects that carry into the future.

Ironically, this contradiction is clearly spelled out in some of the trade-off literature as an intentional assumption. For example, Corbett-Davies et al.~\cite{corbettdavies2017cost} explicitly states: ``Among the rules that satisfy a chosen fairness criterion, we assume policymakers would prefer the one that maximizes immediate utility.'' They intentionally examine the ``proximate costs and benefits'' of the fairness-accuracy trade-off, assuming that this is the temporal resolution that would be most useful to policymakers. This approach enables simplifying mathematical assumptions, as it does not require evaluating how the specific automated decision under consideration has potential ramifications in the future. In Corbett-Davies et al.~\cite{corbettdavies2017cost}, in which they examine risk-assessment decisions for granting bail, they specifically do not need to look at how the immediate decision to detain someone may in fact be predictive of (or even causally linked to) future arrests.  However, if such decisions are applied unfairly across racial demographic groups (even if somewhere slightly ``fairer'' on the optimization curve), then they would just repeat patterns of bias existing in past data.

\subsection{Unfairness of ``Active Fairness'' Trade-Off Remedies}

Some work regarding the fairness-accuracy trade-off sometimes goes beyond observing, characterizing, or implementing the trade-off for different applications, as we have discussed above. They note that while they agree with the notion that the trade-off is inherent, its effects can perhaps be mitigated by increasing \emph{both} accuracy and fairness --- essentially, moving the trade-off optimization curve up and to the right (Figure \ref{fig:optimization}). The trade-off still exists in this scenario, but perhaps is less of an issue since the models perform better overall in terms of both accuracy and fairness.

Concretely, authors recommend a technique they call \emph{active feature acquisition} or \emph{active fairness} \cite{noriegacampero2019active}, which promotes the idea that ``data collection is often a means to reduce discrimination without sacrificing accuracy''  \cite{chen2018tradeoff} --- that collecting more features \emph{for the unprivileged group} will help ensure fairer outcomes \cite{dutta2020tradeoff,bakker2019active}. The rationale is that additional feature collection alleviates the bias in the existing data for unprivileged groups, which will result in reduced bias in the classification results for those groups. Moreover, the authors note that gathering more features for the unprivileged group leads to these benefits without impacting the privileged group; the privileged group's accuracy and fairness metrics remain unchanged.

Setting aside that it might not even be possible to collect more features in practice, there are important implicit assumptions in this choice of solution. In particular, it seems like this work poses data collection as a value-neutral solution to ensure greater fairness. This assumption is clearly false. It is widely accepted, particularly in sociotechnical literature, that data collection is often a form of surveillance \cite{zuboff2018capitalism,clarke1994surveillance,brayne2017surveillance,cohen2011surveillance}. It is not a neutral act, and is generally not equally applied across demographic groups in the US. 

The choice to collect more data raises a normative question directly in contradiction with their goal for increased fairness for unprivileged groups: Do we really want to collect more data on unprivileged groups --- groups that already tend to be surveilled at higher rates than those with more privilege? In the US in particular there is a long history of tracking non-white and queer individuals: Black Americans, from Martin Luther King to Black Lives Matter activists; Japanese Americans during World War II; non-white Muslims, particularly since 9/11; Latine individuals in relation to immigration status; trans, particularly trans-feminine, people in sports and bathroom use \cite{bedoya2016surveillance,desilver2020surveillance,speri2019surveillance,painter2011history, conrad2009trans, fl2021transbill}. In a more global treatment of fairness, is it fair to collect more data on these populations just to ensure we are optimizing some local fairness metric?

One could make the argument that machine learning broadly speaking pushes toward greater surveillance. The field is pushing to train larger and larger model specifications, which tend to require training on larger and larger datasets \cite{kaplan2020scaling}. These data-hungry methods in turn require greater data collection and surveillance in general \cite{zuboff2018capitalism}. Yet, the proposed techniques in active fairness to alleviate the fairness-accuracy trade-off stand apart: They \emph{specifically} advocate for increasing data collection of already-surveilled groups. They tend to leave the data for the privileged group untouched in order to decrease classification disparities between groups. This unfairly shifts the burden of producing fair classification results to the unprivileged group, affording the additional privilege (i.e. even less relative surveillance) to the already-privileged group. Put another way, this solution to the fairness-accuracy optimization problem introduces another, unexplored objective function --- an objective function concerning the burden of surveillance, whose solution in this case causes residual unfairness for the marginalized group.

Some work in active fairness does acknowledge that additional data collection is not costless; however, this work often discusses it as a necessary cost for increased fairness rather than investigating it as a potential source for increased unfairness \cite{chen2018tradeoff}. Noriega-Campero et al.~\cite{noriegacampero2019active} states that it would be useful to model the cost of each feature in the dataset, where costs implicate monetary, privacy, and opportunity concerns. Beyond noting this idea, they do not attempt to formalize it in their work. 

Bakker et al.~\cite{bakker2019active} goes a step further by including cost in their problem formulation, associating a vector of costs with each feature. However, it is unclear how they pick the values of those costs and, perhaps more importantly, they make the assumption that the vector is the same for each individual in the population. This assumes that different values for different features do not not incur different social impacts, which is demonstrably not the case. For example, consider transgender individuals: Trans people, in comparison to cis people, face significant discrimination in response to disclosing their gender identity. In the language of Bakker et al.~\cite{bakker2019active}, it is more costly to trans people to collect features about gender identity than it is for cis people. In fact, such disparate costs can be thought of as the basis for needing to acknowledge and do policymaking using protected demographic attributes in the first place.
