# Supplementary material for: Between Randomness and Arbitrariness: Some Lessons for Reliable Machine Learning at Scale
Source: arXiv:2406.09548 source file (2024-08-12)
Supplement: Supplementary file 6 [file 50-app-emergent-toward-conclusion.tex]

\section{Toward a Resolution} \label{app:sec:emergent:resolution}

\subsection{Making Normative Assumptions Explicit}

Writing mathematical proofs requires assumptions. For example, in machine learning, when writing proofs about an algorithm's properties, it is common to assume that the distribution we are trying to learn is convex. Assumptions like this enable us to guarantee certain logical conclusions about an algorithm's behavior, such as bounds on its convergence rate. While fairness-accuracy trade-off researchers are accustomed to stating mathematical assumptions like this, and ensuring that sound mathematical conclusions follow, we have shown that they do not pay similar attention to normative assumptions and their ensuing contradictory conclusions. We contend that researchers should take the time to make explicit such assumptions underlying their work. Being rigorous and clear about normative assumptions enables them to be reviewed just as rigorously as mathematical assumptions. 

We do not suggest that making such assumptions explicit is a sufficient solution on its own. Nevertheless, it would help facilitate greater scrutiny about the appropriateness of proposed algorithmic fairness solutions. For example, as we discussed in Section \ref{app:sec:emergent:sociotechnical}, this would allow for considering that fairness and accuracy could in fact be in accord \cite{hellman2019fairness, selbst2019abstraction}. ML researchers should engage the assistance of social scientists if they believe they lack the expertise to do this work independently. Moreover, this process should facilitate researchers being introspective about how their individual backgrounds might inform the assumptions they bring into their work. This would be one necessary (though not on its own sufficient) way to address critics of fairness research being dominated by white voices \cite{abdurahman2019response}.

Moreover, clarifying implicit normative assumptions could facilitate rethinking how we measure accuracy. As we note in Section \ref{app:sec:emergent:assumptions}, common accuracy metrics are tied to unfairness. In an attempt to decouple accuracy from unfairness, one could, for example, put a Bayesian prior on existing unfairness and try to correct for it. To the best of our knowledge, no algorithmic fairness scholarship has attempted to do this: to explicitly assume and model the existing unfairness due to a history of discrimination against certain demographics.\footnote{Such modeling, of course, would not come without concern, as it would require introducing a different set of mathematical modeling assumptions that carry their own normative implications.}

\subsection{Tweaking Normative Assumptions for Robustness}

Making normative assumptions explicit could also help facilitate more robust ML fairness research. When investigating algorithmic robustness, researchers are generally comfortable with relaxing or changing certain mathematical proof assumptions and reasoning out the resulting changes (or stasis) in algorithm behavior.  As the economist Edward Leamer~\citep{leamer1983econ} notes:

\begin{quote}
...an inference is not believable if it is fragile, if it can be reversed by minor changes in assumptions. … A researcher has to decide which assumptions or which sets of alternative assumptions are worth reporting.
\end{quote}

As a test of normative robustness, we similarly recommend that fairness-accuracy trade-off researchers perturb their normative assumptions and investigate how this may alter normative outcomes. For example, when considering surveillance of the unprivileged via active feature acquisition as an appropriate mechanism for alleviating the trade-off, it would be useful to state this as an explicit assumption, and then consider surveillance as a constraint for the problem. In other words, one could ask, how much surveillance is tolerable for increased fairness? Perhaps none, but perhaps there is a small set of high quality features that could be collected to serve this purpose, rather than just indiscriminately collecting a lot of additional features.

\section{Conclusion: Reconsidering the Fairness-Accuracy Trade-off} \label{app:sec:emergent:conclusion}
Passi and Barocas \cite{passi2019formulation} note, ``Whether we consider a data science project fair often has as much to do with the formulation of the problem as any property of the resulting model.'' Furthermore, the work of problem formation is ``rarely worked out with explicit normative considerations in mind'' \cite{passi2019formulation}. As we have shown in this article, not attending explicitly to these considerations can lead to contradictory, unintended results: Formulating a trade-off between fairness and accuracy involves a variety of normative assumptions that can in fact lead to various forms of emergent unfairness. 

Our recommendations in Section \ref{app:sec:emergent:resolution} to make normative assumptions explicit aim to remedy this particular type of unfair outcome. However, we recognize that in the case of the fairness-accuracy trade-off, fully applying these recommendations may not be sufficient in itself. Rather, in clarifying the normative concerns of the trade-off, it is quite possible to reasonably conclude that the effects of emergent unfairness outweigh any benefits that come from choosing this particular problem formulation. As such, when it comes to the critical issue of algorithmic fairness, it may be time to reconsider the framing of trade-offs altogether.
